# Supplementary material for: Price of Anarchy for Auction Revenue
Source: arXiv:1404.5943 source file (2019-01-16)
Supplement: Supplementary file 3 [file appendix-reserves.tex]

\section{Reserves Extension}
\label{sec:appres}

\label{sec:res}
Consider adding arbitrary bidspace reserves $\reserves$ to a first-price auction. Deriving a revenue result with our framework required two properties: (1) reserves prevented profitable allocation to low-valued agents and (2) we preserved the structure of the auction for bids above the reserve (and therefore preserved revenue covering). Property (1), along with regularity, implied virtual value covering, which combined with the revenue covering from (2) to produce a revenue bound. We seek to capture these two properties when defining reserves for general mechanisms.

\begin{definition}
\label{def:res}
For a mechanism $\mech$, let $\mechr$ be $\mech$ restricted to an action space $A^{\reserves}$. We say $\mechr$ \emph{implements $\mech$ with covering-preserving reserves $\reserves=(r_1,\ldots,r_n)$} if the following hold:
\begin{enumerate}
%\item No agent with value $\valagent<\reserveagent$ is allocated in any BNE of $\mechr$.
\item For any strategy profile $\strat$, and any bidder $i$, 
\begin{enumerate}
\item Every action $\actionagent\in A_i^{\reserves}$ has $\equivbid_\agent(\actionagent)\geq \reserveagent$.
\item Either there is a \emph{reserve action} $\actionagent^{\reserveagent}\in A_i^{\reserves}$ with $\equivbid_i(\actionagent^{\reserveagent}) = \reserveagent$ or there is no action with positive probability of winning and equivalent bid at most $\reserveagent$ in $\mech$.
\end{enumerate}
\item There exists a set $\mathbf{A'}$ such that $\mech$ is $\mu$-revenue covered restricted to the action sets $\mathbf A^{\reserves}\cap\mathbf{A'}$ for bidders with values $\vals\geq \reserves$. We say the reserves respect $\mathbf A'$
%\item\label{defpart:struc} For every strategy profile $\stratres$ in $\mechr$, there exists a strategy profile $\strat$ in $\mech$ such that:
%
% \begin{enumerate}
%\item \label{defpart:rev} $\bidpayment(\strat(\val))=\bidpaymentr(\stratres(\val))$ and $\bidalloc(\strat(\val))=\bidallocr(\stratres(\val))$ for all value profiles $\val$.
%%\item \label{defpart:mins} $\allocrmin\geq\allocmin$.
%\item \label{defpart:thresh} There is a restricted action set $\actspacealt$ in $\mech$ such that for each agent $\agent$, if $\allocdev\geq\allocrmin$, then $\thresholdragent(\allocdev)\leq\thresholdagentrest(\allocdev)$. We say $\mechr$ \emph{respects} $\actspacealt$.
\end{enumerate}
\end{definition}

Note that this definition does not naturally capture the addition of reserves in such mechanisms as the second-price auction. In particular, for that auction, the addition of reserves increases expected payments for agents, so condition revenue covering isn't obviously preserved in the reserves mechanism. Second-price auctions are not revenue covered, as we show in Section~\ref{sec:spa}, so this is less concerning. The definition does, however, capture the addition of reserves in auctions with first-price payment semantics.

Adding arbitrary reserves $\reserves$ to a $\revpar$-revenue covered mechanism in the manner of Definition~\ref{def:res} preserves revenue covering. Formally:

\begin{lemma}
\label{lem:reservesextension}
Let $\mechr$ implement a mechanism $\mech$ with covering-preserving reserves $\reserves$ which respect restricted actions $\actspacealt$, and let $S^\reserves$ map value profiles to agents for which $\valagent\geq\reserveagent$. If $\mech$ is $\revpar$-revenue covered with respect to $\actspacealt$, then $\mechr$ is $\revpar$-revenue covered with respect to $S^\reserves$.
\end{lemma}

Lemma~\ref{lem:reservesextension} implies that revenue covered mechanisms with reserves added are still revenue covered. We can therefore use Theorem~\ref{thm:reswel} to bound the welfare of the reserves mechanism.

\begin{theorem}
Let $\mechr$ implement a mechanism $\mech$ with individual reserves $\reserves$. If $\mech$ is $\revpar$-revenue covered, then in any BNE of $\mechr$, the welfare of $\mechr$ is a $(1+\revpar)\frac{e}{e-1}$-approximation to the welfare of any other mechanism which only serves agents with $\valagent\geq\reserveagent$.
\end{theorem}

In particular, we have that the first-price auction with reserves $\reserves$ in bidspace approximates the welfare of the optimal mechanism which only serves agents with $\valagent\geq\reserveagent$, which is $\VCG$ with reserves $\reserves$. Furthermore, we show in Section~\ref{sec:simul} that the simultaneous composition of several first-price auctions is revenue covered.
