# Supplementary material for: Price of Anarchy for Auction Revenue
Source: arXiv:1404.5943 source file (2019-01-16)
Supplement: Supplementary file 6 [file appendix-simultaneous.tex]

\section{Simultaneous Composition Proofs}\label{sec:appsim}
We prove revenue covering holds under simultaneous composition by proving a stronger notion of revenue covering holds, revenue covering when bidders have a restricted set of actions they can take. We consider thresholds derived from participating in only one of the mechanisms being composed. These thresholds will retain the revenue covering properties of the original mechanisms and cause the global mechanism to inherit the property as well.

Given a strategy $\strat$ in the composed mechanism, let $\stratitem$ denote the strategy profile in mechanism $\mitem$ defined by the element of each agent's strategy profile corresponding to $\mechitem$. Given $\stratitem$, define $\thresholdagentitem$, and $T_\agent^\mitem$ to be the analogous values of $\thresholdagent$, and $T_\agent$ in $\mechitem$ under $\stratitem$. In the composed mechanism, let $\actspaceagentitem$ be the set of actions comprised of an arbitrary action in mechanism $\mitem$ and withdrawing from all other mechanisms. Further let $\actspaceagentalt=\bigcup_\mitem \actspaceagentitem$, and $\actspacealt=\prod_\agent \actspaceagentalt$.

\paragraph{Action Restrictions} 
Restricting the set of allowed actions by bidders only decreases their allocation for any equivalent bid and hence only increases their threshold. It follows that if a mechanism's revenue covers the cumulative threshold derived from a restricted action set, then it also covers those from the unrestricted action set. The following are analogous to the original definitions, but with a restricted action set:

\begin{definition}
The equivalent threshold bid with respect to a restricted action set $\actspaceagentalt\subseteq \actspaceagent$, denoted $\thresholdagentrest(\allocdev)$, is defined as $\min_{\actionagent\in\actspaceagentalt} \equivbidagent(\actionagent)$ subject to $\bidallocagent(\actionagent)\geq \allocdev$.
\end{definition}
\begin{definition}
Given an action $\actionagent$, the expected equivalent threshold bid with respect to a restricted action set $\actspaceagentalt\subseteq\actspaceagent$, denoted $\threshexpectedrest{\bidallocagent(\actionagent)}{\allocaltagent},$ is defined as $\int_{\bidallocagent(\actionagent)}^{\alloclevel}\thresholdagentrest(\allocdev)\,d\allocdev.$
\end{definition}
%Note that the lower limit of the integral is $\allocmin$, still defined with respect to the full action set $\actspaceagent$.
%\begin{definition}
%\label{def:RRC}
%A mechanism $\mech$ is $\revpar$-revenue covered with respect to action set restrictions $A_1'(\strat)\subseteq A_1,\ldots,A_n'(\strat)\subseteq A_n$ (with product space $\actspacealt(\strat)$) if for every strategy profile $\strat$, alternate feasible allocation $\allocalt$, and profile of general actions $\actions$, $\revpar\rev(\mech) \geq \sum\nolimits_\agent\threshexpactions{A_i'(\strat)}{\bidallocagent(\actionagent)}{\allocaltagent}$.
%\end{definition}

\begin{definition}
\label{def:RRC}
A mechanism $\mech$ is $\revpar$-revenue covered restricted to actions $A_1'\subseteq A_1,\ldots,A_n'\subseteq A_n$ (with product space $\actspacealt$) if for every strategy profile $\strat$, alternate feasible allocation $\allocalt$, and profile of general actions $\actions$, $\revpar\rev(\mech) \geq \sum\nolimits_\agent\threshexpectedrest{\bidallocagent(\actionagent)}{\allocaltagent}$.
\end{definition}

Note that restricted revenue covering is stronger than unrestricted revenue covering, and as such proving a mechanism is revenue covered for a given restriction is sufficient to show that it is revenue covered with no restriction. This follows from the fact that $\thresholdagentrest(\allocdev)$ is the objective value to the same minimization problem as $\thresholdagent(\allocdev)$, but on a smaller feasible region, so $\thresholdagentrest(\allocdev)\geq\thresholdagent(\allocdev)$ for all $\agent$ and $\allocdev$. Integrating, we see that $\threshexpectedrest{\bidallocagent(\actionagent)}{\allocaltagent}\geq\threshexpected{\bidallocagent(\actionagent)}{\allocaltagent}$ for all $\agent$ and $\alloclevel$, so $\rev(\mech)\geq\sum\nolimits_\agent\threshexpectedrest{\bidallocagent(\actionagent)}{\allocaltagent}\geq\sum\nolimits_\agent\threshexpected{\bidallocagent(\actionagent)}{\allocaltagent}.$ %These definitions can be further adapted to handle restricted action sets which depend on the strategy profile, i.e. $\actspacealt(\strat)=A_1'(\strat),\ldots,A_n'(\strat)$.

Additionally, restricted revenue covering combines with revenue covering for bidders with values above a set of reserves (Definition \ref{def:revcoverabove}) in the logical manner, only summing over bidders with values above reserves.

%\begin{definition}
%\label{def:restricted3}
%Let $\filter$ be a function which takes a value profile $\val$ and outputs a set of agents, and action set restrictions $A_1'(\strat)\subseteq A_1,\ldots,A_n'(\strat)\subseteq A_n$ (with product space $\actspacealt(\strat)$). A mechanism $\mech$ is $\revpar$-revenue covered with respect to $\filter$ and $\actspacealt(\strat)$ if for all alternate allocations $\allocalt$, value profiles $\val$, and profiles of participatory actions $\actions$,
%\begin{equation*}
%\revpar\rev(\mech)\geq\sum\nolimits_{\agent\in\filter(\val)} \threshexpectedrest{\bidallocagent(\actionagent)}{\allocaltagent}.
%\end{equation*}
%\end{definition}
%Revenue covering in the sense of Definition~\ref{def:restricted3} implies that in the sense of Definition~\ref{def:restricted2}.

\restate{Lemma~\ref{lem:seq}}{
Let $\mech$ be the simultaneous composition of $\revpar$-revenue covered (with reserves $\reserves$) mechanisms $\mech_1, \ldots \mech_m$ with unit-demand, single-valued agents. Then $\mech$ is $\revpar$-revenue covered (with reserves $\reserves$).}

\begin{proof}
We prove that $\mech$ is $\revpar$-revenue covered with respect to $\actspacealt$, the restriction to only participating in one mechanism at a time. We will assume for the proof that $\reserves = (0, \ldots, 0)$. We conclude with an explanation of the proof for the non-zero reserves case.

Let $\allocalt$ be a feasible induced allocation for the global mechanism. That is, we can construct a matching between agents and mechanisms such that for any $\mitem$, there is a feasible allocation for $\mechitem$ that allocates each $\agent$ matched to $\mitem$ according to $\allocaltagent$. Define $\allocaltagentitem$ be $\allocaltagent$ if $\agent$ and $\mitem$ are matched, and 0 otherwise. Note that for each agent $\agent$, $\allocaltagentitem>0$ for at most one $\mitem$, with $\allocaltagentitem=0$ for all $\mitem$ if $\allocaltagent=0$. By downward closure, $\allocaltitem$ is a feasible allocation for $\mechitem$.

Now by the definition of the composed mechanism, $\revpar\rev(\mech)=\revpar\sum\nolimits_\mitem\rev(\mechitem),$ where $\rev(\mechitem)$ is taken with respect to $\stratitem$ for each $\mitem$.  Let $\actions$ be an action profile in $\mech$, and let $\actionsitem$ be the corresponding vector of actions in mechanism $\mitem$. Because each $\mechitem$ is $\revpar$-revenue covered, it follows that $\revpar\sum\nolimits_\mitem\rev(\mechitem)\geq\sum\nolimits_\mitem\sum_\agent\threshexpecteditem{\bidallocagentitem(\actionagentitem)}{\allocaltagentitem}$.  Moreover, for all $\mitem$, $\threshexpecteditem{\bidallocagentitem(\actionagentitem)}{\allocaltagentitem}=\expthresholdagent^{\actspaceagentitem}[\bidallocagentitem(\actionagentitem),\allocaltagentitem]\geq\expthresholdagent^{\actspaceagentalt}[\bidallocagentitem(\actionagentitem),\allocaltagentitem]$, and by the definition of the induced single-dimensional allocation rule of the composed mechanism, $\simallocagent$, $\expthresholdagent^{\actspaceagentalt}[\bidallocagentitem(\actionagentitem),\allocaltagentitem]\geq\expthresholdagent^{\actspaceagentalt}[\simallocagent(\actionagent),\allocaltagentitem]$. But for each agent $\agent$, $\allocaltagentitem>0$ for at most one $\mitem$, so $\threshexpecteditem{\bidallocagentitem(\actionagentitem)}{\allocaltagentitem}>0$ for at most one $\mitem$ as well, again with $\threshexpecteditem{\bidallocagentitem(\actionagentitem)}{\allocaltagentitem}=0$ for all $\mitem$ if $\allocaltagent=0$. The same also holds for $\expthresholdagent^{\actspaceagentalt}[\simallocagent(\actionagent),\allocaltagentitem]$. It follows that $\sum\nolimits_\mitem\sum_\agent\threshexpecteditem{\bidallocagentitem(\actionagentitem)}{\allocaltagentitem}\geq\sum\nolimits_\agent \expthresholdagent^{\actspaceagentalt}[\simallocagent(\actionagent),\allocaltagentitem]$, which implies the result.

\end{proof}

The proof with nonzero reserves differs slightly from the above in two ways. First, we consider the thresholds only of agents with values above their reserves. As above, the proof compares the thresholds of these agents in the global mechanism to those of the local mechanisms. Second, given a participatory action profile $\actions$ for the global mechanism, we need only consider thresholds from mechanisms where $\actionagentitem$ is also participatory. As reserves are the same across all mechanisms, the local cumulative thresholds above the allocation from a participatory action are larger than those for the global mechanism for the same allocation, giving the same result.
